# Supplementary material for: $\nabla^2$DFT: A Universal Quantum Chemistry Dataset of Drug-Like Molecules and a Benchmark for Neural Network Potentials
Source: arXiv:2406.14347 source file (2024-12-13)
Supplement: Supplementary file 1 [file XX_supplementary_materials.tex]

%\begin{landscape}
\begin{table}[]
\caption{Summary of quantum chemistry dataset. (+) denotes information that is not provided in a direct way in article or descriptions. (*) denotes parameters that can be derived from dataset with some computation.}\label{tbl:dataset-summary}
\tiny
\addtolength{\tabcolsep}{-1pt} 
\begin{tabular}{llllllllll} \hline
                                                                   & \textbf{NablaDFT2}                                                               & \textbf{NablaDFT}                                                                  & \textbf{QM7}                                                                                & \textbf{QM7b}                                                                                   & \textbf{QM7-X}                                                                          & \textbf{QM9}                                                                            & \textbf{\begin{tabular}[c]{@{}l@{}}MultiXC-\\ QM9\end{tabular}}                          & \textbf{QM1B}                                                          & \textbf{QH9}                                                                                      \\ \hline
\begin{tabular}[c]{@{}l@{}}Chem. inf.\\ Source\end{tabular}        & \begin{tabular}[c]{@{}l@{}}MOSES,\\ ZINC21\\ (Zinc\\ Clean\\ Leads)\end{tabular} & \begin{tabular}[c]{@{}l@{}}MOSES,\\ ZINC21\\ (Zinc \\ Clean \\ Leads)\end{tabular} & GDB-13                                                                                      & GDB-13                                                                                          & GDB-13                                                                                  & GDB-17                                                                                  & GDB-17                                                                                   & GDB-11                                                                 & \begin{tabular}[c]{@{}l@{}}GDB-13, \\ QM9\end{tabular}                                            \\
\begin{tabular}[c]{@{}l@{}}\# of\\ molecules\end{tabular}          & 2M                                                                               & 1M                                                                                 & 7K                                                                                          & 7K                                                                                              & 7K                                                                                      & 134K                                                                                    & 134K                                                                                     & 1M                                                                     & 130K                                                                                              \\
\begin{tabular}[c]{@{}l@{}}\# of \\ conformers\end{tabular}        & 13M                                                                              & 5M                                                                                 & 7K                                                                                          & 7K                                                                                              & 4M                                                                                      & 134K                                                                                    & 134K                                                                                     & 1B                                                                     & 130K                                                                                              \\
\begin{tabular}[c]{@{}l@{}}\# of \\ atoms\end{tabular}             & 8-62                                                                             & 8–62                                                                               & 1-23                                                                                        & 1-23                                                                                            & 1-23                                                                                    & 3-29                                                                                    & 3-29                                                                                     & 9-11                                                                   & 3-29                                                                                              \\
\begin{tabular}[c]{@{}l@{}}\# of \\ heavy \\ atoms\end{tabular}    & 8-27                                                                             & 8–27                                                                               & 1-7                                                                                         & 1-7                                                                                             & 1-7                                                                                     & 1-9                                                                                     & 1-9                                                                                      & +                                                                      & 1-9\\
Atoms                                                              & \begin{tabular}[c]{@{}l@{}}H,C,N,\\ O,S, Cl,\\ F,Br\end{tabular}                 & \begin{tabular}[c]{@{}l@{}}H,C,N,\\ O,Cl,F,\\ Br\end{tabular}                      & \begin{tabular}[c]{@{}l@{}}H,C,N,\\ O,S\end{tabular}                                        & \begin{tabular}[c]{@{}l@{}}H,C,N,\\ O,S\end{tabular}                                            & \begin{tabular}[c]{@{}l@{}}H,C,N,\\ O,S,Cl\end{tabular}                                 & \begin{tabular}[c]{@{}l@{}}H,C,N,\\ O,F\end{tabular}                                    & \begin{tabular}[c]{@{}l@{}}H,C,N,\\ O,F\end{tabular}                                     & \begin{tabular}[c]{@{}l@{}}H,C,N,\\ O,F\end{tabular}                   & \begin{tabular}[c]{@{}l@{}}H,C,N,\\ O,F\end{tabular}                                              \\
\begin{tabular}[c]{@{}l@{}}Forces\end{tabular}             & Yes                                                                              & Yes                                                                                & No                                                                                          & No                                                                                              & Yes                                                                                     & No                                                                                      & No                                                                                       & No                                                                     & Yes                                                                                               \\
\begin{tabular}[c]{@{}l@{}}Hamilt-\\onians\end{tabular}                                                   & Yes                                                                              & Yes                                                                                & No                                                                                          & No                                                                                              & No                                                                                      & No                                                                                      & No                                                                                       & No                                                                     & No                                                                                                \\
\begin{tabular}[c]{@{}l@{}}Optim\\ traj.\end{tabular}              & Yes                                                                              & No                                                                                 & No                                                                                          & No                                                                                              & No                                                                                      & No                                                                                      & No                                                                                       & No                                                                     & Yes                                                                                               \\
\begin{tabular}[c]{@{}l@{}}Basis set\\ and\\ XC-func.\end{tabular} & \begin{tabular}[c]{@{}l@{}}$\Omega$B97X-\\ D/\\ Def2-\\ SVP\end{tabular}         & \begin{tabular}[c]{@{}l@{}}$\Omega$B97X-\\ D/\\ Def2-\\ SVP\end{tabular}           & PBE0                                                                                        & \begin{tabular}[c]{@{}l@{}}ZINDO, \\ SCS, \\ PBE0, \\ GW\end{tabular}                           & \begin{tabular}[c]{@{}l@{}}ePBE0+\\ MBD, \\ TotFOR\end{tabular}                         & \begin{tabular}[c]{@{}l@{}}B3LYP/6-\\ 31G(2df,p)\\ + G4MP2\end{tabular}                 & \begin{tabular}[c]{@{}l@{}}B3LYP and PBE/\\ 6–31G(2df,p),\\ SZ, DZP,\\ TZP\end{tabular} & \begin{tabular}[c]{@{}l@{}}STO-3G/\\ B3LYP\end{tabular}                & \begin{tabular}[c]{@{}l@{}}B3LYP/\\ Def2SVP\end{tabular}                                          \\
\begin{tabular}[c]{@{}l@{}}Storage\\ size\end{tabular}             & 220 Tb                                                                           & 100 Tb                                                                             & 17.9 MB                                                                                     & 16.1 MB                                                                                         & 1.35 Gb                                                                                 & 230 Mb                                                                                  & 317 Gb                                                                                   & 240 GB                                                                 & 28.4 Gb                                                                                           \\ \hline
                                                                   & \textbf{GEOM}                                                                    & \textbf{ANI-1}                                                                     & \textbf{\begin{tabular}[c]{@{}l@{}}ANI-1x/\\ ANI-1cxx\end{tabular}}                         & \textbf{\begin{tabular}[c]{@{}l@{}}OrbNet\\ Denali\end{tabular}}                                & \textbf{QMugs}                                                                          & \textbf{SPICE}                                                                          & \textbf{PubChemQC}                                                                       & \textbf{Frag20}                                                        & \textbf{VQM24}                                                                                    \\ \hline
\begin{tabular}[c]{@{}l@{}}Chem. inf.\\ Source\end{tabular}        & \begin{tabular}[c]{@{}l@{}}QM9,\\ AICures\end{tabular}                           & GDB                                                                                & \begin{tabular}[c]{@{}l@{}}GDB-11,\\ ChEMBL\end{tabular}                                    & ChEMBL27                                                                                        & ChEMBL                                                                                  & \begin{tabular}[c]{@{}l@{}}PubChem+\\ DES370K+\\ Other\end{tabular}                     & PubChem                                                                                  & \begin{tabular}[c]{@{}l@{}}PubChem,\\ ZINC\end{tabular}                & \textit{\begin{tabular}[c]{@{}l@{}}Combi- \\ natorial\end{tabular}}                               \\
\begin{tabular}[c]{@{}l@{}}\# of\\ molecules\end{tabular}          & 450K                                                                             & 57K                                                                                & 57K                                                                                         & 16K                                                                                             & 665K                                                                                    & 19K                                                                                     & 85M                                                                                      & 565K                                                                   & 10K                                                                                               \\
\begin{tabular}[c]{@{}l@{}}\# of \\ conformers\end{tabular}        & 37M                                                                              & 24M                                                                                & 20M                                                                                         & 2.3M                                                                                            & 2M                                                                                      & 1KK                                                                                     & 85M                                                                                      & 566K                                                                   & 835K                                                                                              \\
\begin{tabular}[c]{@{}l@{}}\# of \\ atoms\end{tabular}             & +                                                                                & +                                                                                  & 2-26                                                                                        & +                                                                                               & 4-228                                                                                   & 2–96                                                                                    & +                                                                                        & +                                                                      & 4,5                                                                                               \\
\begin{tabular}[c]{@{}l@{}}\# of \\ heavy \\ atoms\end{tabular}    & +                                                                                & 1-11                                                                               & 1-8                                                                                         & +                                                                                               & 4-100                                                                                   & +                                                                                       & 51                                                                                       & 20                                                                     & +                                                                                                 \\
Atoms                                                              & \begin{tabular}[c]{@{}l@{}}H,C,N,\\ O,F,+\end{tabular}                           & \begin{tabular}[c]{@{}l@{}}H,C,N,\\ O\end{tabular}                                 & \begin{tabular}[c]{@{}l@{}}H,C,N,\\ O\end{tabular}                                          & \begin{tabular}[c]{@{}l@{}}H,Li,B,\\ C,N,O,\\ F,Na,Mg,\\ Si,P,S,\\ Cl,K,Ca,\\ Br,I\end{tabular} & \begin{tabular}[c]{@{}l@{}}H,C,N,\\ O,P,S,\\ Cl,F,Br,\\ I\end{tabular}                  & \begin{tabular}[c]{@{}l@{}}H,Li,C,\\ N,O,F,\\ Na,Mg,P,\\ S,Cl,K,\\ Ca,Br,I\end{tabular} & \begin{tabular}[c]{@{}l@{}}H,C,N,\\ O,P,S, \\ F,Cl,Na\\ K,Mg,Ca,\end{tabular}            & \begin{tabular}[c]{@{}l@{}}H,B,C,\\ O,N,F,\\ P,S,Cl,\\ Br\end{tabular} & \begin{tabular}[c]{@{}l@{}}H,C,N,\\ O,F,Si,\\ P,S,Cl,\\ Br\end{tabular}                           \\
\begin{tabular}[c]{@{}l@{}}Forces\end{tabular}             & Yes                                                                              & No                                                                                 & No                                                                                          & No                                                                                              & No*                                                                                     & Yes                                                                                     & No                                                                                       & No                                                                     & No                                                                                                \\
\begin{tabular}[c]{@{}l@{}}Hamilt-\\onians\end{tabular}         & No                                                                               & No                                                                                 & No                                                                                          & No                                                                                              & No*                                                                                     & No                                                                                      & No                                                                                       & No                                                                     & No                                                                                                \\
\begin{tabular}[c]{@{}l@{}}Optim\\ traj.\end{tabular}              & No                                                                               & No                                                                                 & No                                                                                          & No                                                                                              & No                                                                                      & No                                                                                      & No                                                                                       & No                                                                     & No                                                                                                \\
\begin{tabular}[c]{@{}l@{}}Basis set\\ and\\ XC-func.\end{tabular} & \begin{tabular}[c]{@{}l@{}}mTZVPP/\\ R2scan-3\end{tabular}                       & \begin{tabular}[c]{@{}l@{}}WB97x/\\ 6–31g(d)\end{tabular}                          & \begin{tabular}[c]{@{}l@{}}wB97x/\\6-31G*, \\ wB97x/\\def2-TZVPP, \\ CCSD(T)*/\\CBS,\end{tabular} & \begin{tabular}[c]{@{}l@{}}$\Omega$B97X-\\ D3/\\ Def2-\\ TZVP\end{tabular}                      & \begin{tabular}[c]{@{}l@{}}$\omega$B97X-\\ D/\\ Def2-\\ SVP\\ +GFN2-\\ XTB\end{tabular} & \begin{tabular}[c]{@{}l@{}}$\omega$B97M-\\ D3(BJ)/\\ Def2-\\ TZVPPD\end{tabular}        & \begin{tabular}[c]{@{}l@{}}B3LYP/\\ 6-31G*+\\ PM6\end{tabular}                           & \begin{tabular}[c]{@{}l@{}}B3LYP/\\ 6-31G*\end{tabular}                & \begin{tabular}[c]{@{}l@{}}$\Omega$B97X-D3/\\ Cc-\\ pVDZ,\\ DMC@\\PBE0(cEC/\\ Cc-VQZ))\end{tabular} \\
\begin{tabular}[c]{@{}l@{}}Storage\\ size\end{tabular}             & 130.8 GB                                                                         & 4.48 Gb                                                                            & 5.29 Gb                                                                                     & 2.74 GB                                                                                         & 7 Tb                                                                                    & 37.5 GB                                                                                 & 100 Tb                                                                                   & 566 Mb                                                                 & 1.5 Gb                                                                                  \\\hline    
\end{tabular}
\addtolength{\tabcolsep}{1pt} 
\end{table}

%\end{landscape}

\begin{table}[]
  \caption{Properties available for each data instance in $\nabla^2$DFT.}\label{tbl:properties}
  \footnotesize
\begin{tabular}{cl}
\hline
\multicolumn{1}{c}{Access mode}                                              & \multicolumn{1}{c}{Content}                                       \\ \hline
\begin{tabular}[c]{@{}l@{}}Main data\\ (from basic\\dataloader)\end{tabular}  & \begin{tabular}[c]{@{}l@{}}Atoms numbers, atoms positions, energy ('DFT FORMATION ENERGY'), forces, \\  Hamiltonian (Fock matrix), overlap matrix, coefficients matrix\end{tabular}\\  \hline 
\begin{tabular}[c]{@{}c@{}}Metainformation\\ (from\\summary.csv)\end{tabular} & \begin{tabular}[c]{@{}l@{}}'DFT TOTAL ENERGY', 'DFT XC ENERGY', 'DFT NUCLEAR REPULSION ENERGY', \\ 'DFT ONE-ELECTRON ENERGY', 'DFT TWO-ELECTRON ENERGY', \\ 'DFT DIPOLE X', 'DFT DIPOLE Y', 'DFT DIPOLE Z', 'DFT TOTAL DIPOLE',\\ 'DFT ROT CONSTANT A', 'DFT ROT CONSTANT B', 'DFT ROT CONSTANT C',\\ 'DFT HOMO', 'DFT LUMO', 'DFT HOMO-LUMO GAP', \\ 'DFT ATOMIC ENERGY', 'DFT FORMATION ENERGY'\end{tabular}                                                                               \\  \hline
\begin{tabular}[c]{@{}c@{}}Raw stored\\ wavefunction\\ object\end{tabular}   & \begin{tabular}[c]{@{}l@{}}All DATA FROM TWO PREVIOUS ROWS, \\ Ca/Cb (molecular orbital coefficients), Da/Db (density matrix), Fa/Fb (Fock matrix), \\ H (Core Hamiltonian), S (overlap matrix), X (XC-functional matrix), \\ aotoso (Atomic Orbital to Symmetry Orbital), epsilon\_a/epsilon\_b (orbital eigenvalues), \\ SCF DIPOLE, doccpi (number of doubly occupied orbitals), nmo (number of molecule orbitals),\\ 'DISPERSION CORRECTION ENERGY', 'GRID ELECTRONS TOTAL'\end{tabular} \\  \hline
\begin{tabular}[c]{@{}l@{}}Available after \\ loading into Psi4\end{tabular} & \begin{tabular}[c]{@{}l@{}}All DATA FROM THREE PREVIOUS ROWS, \\ Electric dipole moment, Electric quadrupole moment, All moments up order N, \\ Electrostatic potential at nuclei, Electrostatic potential on grid, Electric field on grid, \\ Molecular orbital extents, Mulliken atomic charges, Löwdin atomic charges, \\ Wiberg bond indices, Mayer bond indices, Natural orbital occupations, \\ Stockholder Atomic Multipoles, Hirshfeld volume ratios\end{tabular}                    \\ \hline
\end{tabular}
\end{table}
